# Supplementary material for: Griffon: Spelling out All Object Locations at Any Granularity with Large Language Models
Source: arXiv:2311.14552 source file (2024-10-08)
Supplement: Supplementary file 1 [file supp.tex]

\clearpage
\setcounter{page}{1}
\appendix

\setcounter{section}{0}
This supplementary document expands upon our main paper by offering additional insights into our proposed Language-prompted Detection Dataset, implementation details, and more visualization results, constrained by length limit. In \cref{LPDD}, we delineate the data processing procedure, data reformatting, and instruction template generation, illustrated with examples in \cref{Prompt examples}. The hyperparameter settings for our paper are outlined in \cref{sec: hyper}. Lastly, we employ a demo style to present additional visualization results for various tasks.

\section{Details of Language-prompted Detection Dataset}
\label{LPDD}
{\bf Overall.} After collecting data from public datasets, we further organize, process, and optimize the data, and propose the Language-prompted Detection Dataset. Overall, we have 6M pre-training data and nearly 900K instruction following data. Detailed statistics of the Language-prompted Detection Dataset can be found in \cref{tab:data composition}. 

\begin{table}
    \centering
    \caption{{The statistic of the composition of Language-prompted Detection Dataset.} OD represents object detection, and PG represents the phrase grounding with positive tokens for referents. 1 \vs 1 denotes the Single Referent scenario, n \vs n denotes Multi Categories with Multi Objects scenario, 1 \vs n denotes One Category with Multi Objects, and None denotes None-Existing scenario.}
    \begin{tabular}{c|c|c|c}
        \toprule
         &Vol.&  Type & Source Datasets\\
         \midrule
         \multirow{2}{*}{Pre-training}&4M&REC&RefCOCO, RefCOCO+/g, Visual Genome\\
         &2M&OD&Objects365, MSCOCO\\
         \midrule
         \multirow{4}{*}{Instruction-following}&288K& 1 \vs 1& RefCOCO, RefCOCO+/g\\
         &118K&n \vs n &MSCOCO\\
         &427K& 1 \vs n & Flickr30K Entities\\
         &40K&None&LVIS\\
         \bottomrule
    \end{tabular}
    \label{tab:data composition}
\end{table}
{\bf Data Processing.} The image and annotation processing involves three critical steps to ensure optimal data quality. Initially, we exclude images with a maximum resolution smaller than 250 pixels to prevent adverse effects on training. Subsequently, we rigorously review each image's annotations, discarding those with discrepancies between actual and annotated sizes – a common issue with internet-sourced images. Lastly, we validate the annotations to eliminate inaccuracies, focusing on refining bounding boxes and rectifying incomplete category labels.

{\bf Data Reformatting.} We have tailored our approach to reformat diverse source datasets into a unified language-prompted style, aligning with specific scenarios: 
\begin{itemize}
    % \item For the Single Referent data, leveraging Shikra’s original annotations, we refine GRIT’s caption-based annotations by extracting single referents and discarding multi-object references. This step is crucial to maintain quality, especially given the prevalence of low-quality multi-object annotations. We also balance the GRIT part by retaining all middle and small objects and sampling large objects at a 1:1 ratio.
    \item For the One Category with Multi Objects data, unlike traditional methods using Flickr30K Entities that focus on caption-based object grounding, we extract phrases and their corresponding bounding boxes. Each phrase and its bounding boxes constitute a single annotation, aligning more closely with everyday usage.
    \item For the Non-existing data, we first construct from the LVIS dataset with its negative categories annotations. For each image containing the negative categories, we randomly select one category and pair it with the image to form an entry. Additionally, to increase the variety of the text granularity, we mine negative referents from the attributes of the object such as the color and position with GPT-4V exampled in \cref{fig: Negative mining}.
    \item For the Multi Categories with Multi Objects, we concatenate the annotations of each image in the object detection datasets, ensuring comprehensive coverage of this scenario.
\end{itemize}

{\bf Instruction Templates Generation.} With the reformatted data, we utilize the template generation method proposed in \cref{subsec: data construction} (main paper) to generate various templates for different scenarios. As shown in \cref{tab: template}, we input the information listed in the table to the GPT-4V and the required templates will be returned. We provide some examples of the templates we generate in \cref{fig:templates_demo}.

\begin{figure}
    \centering
    \includegraphics[width=0.5\linewidth]{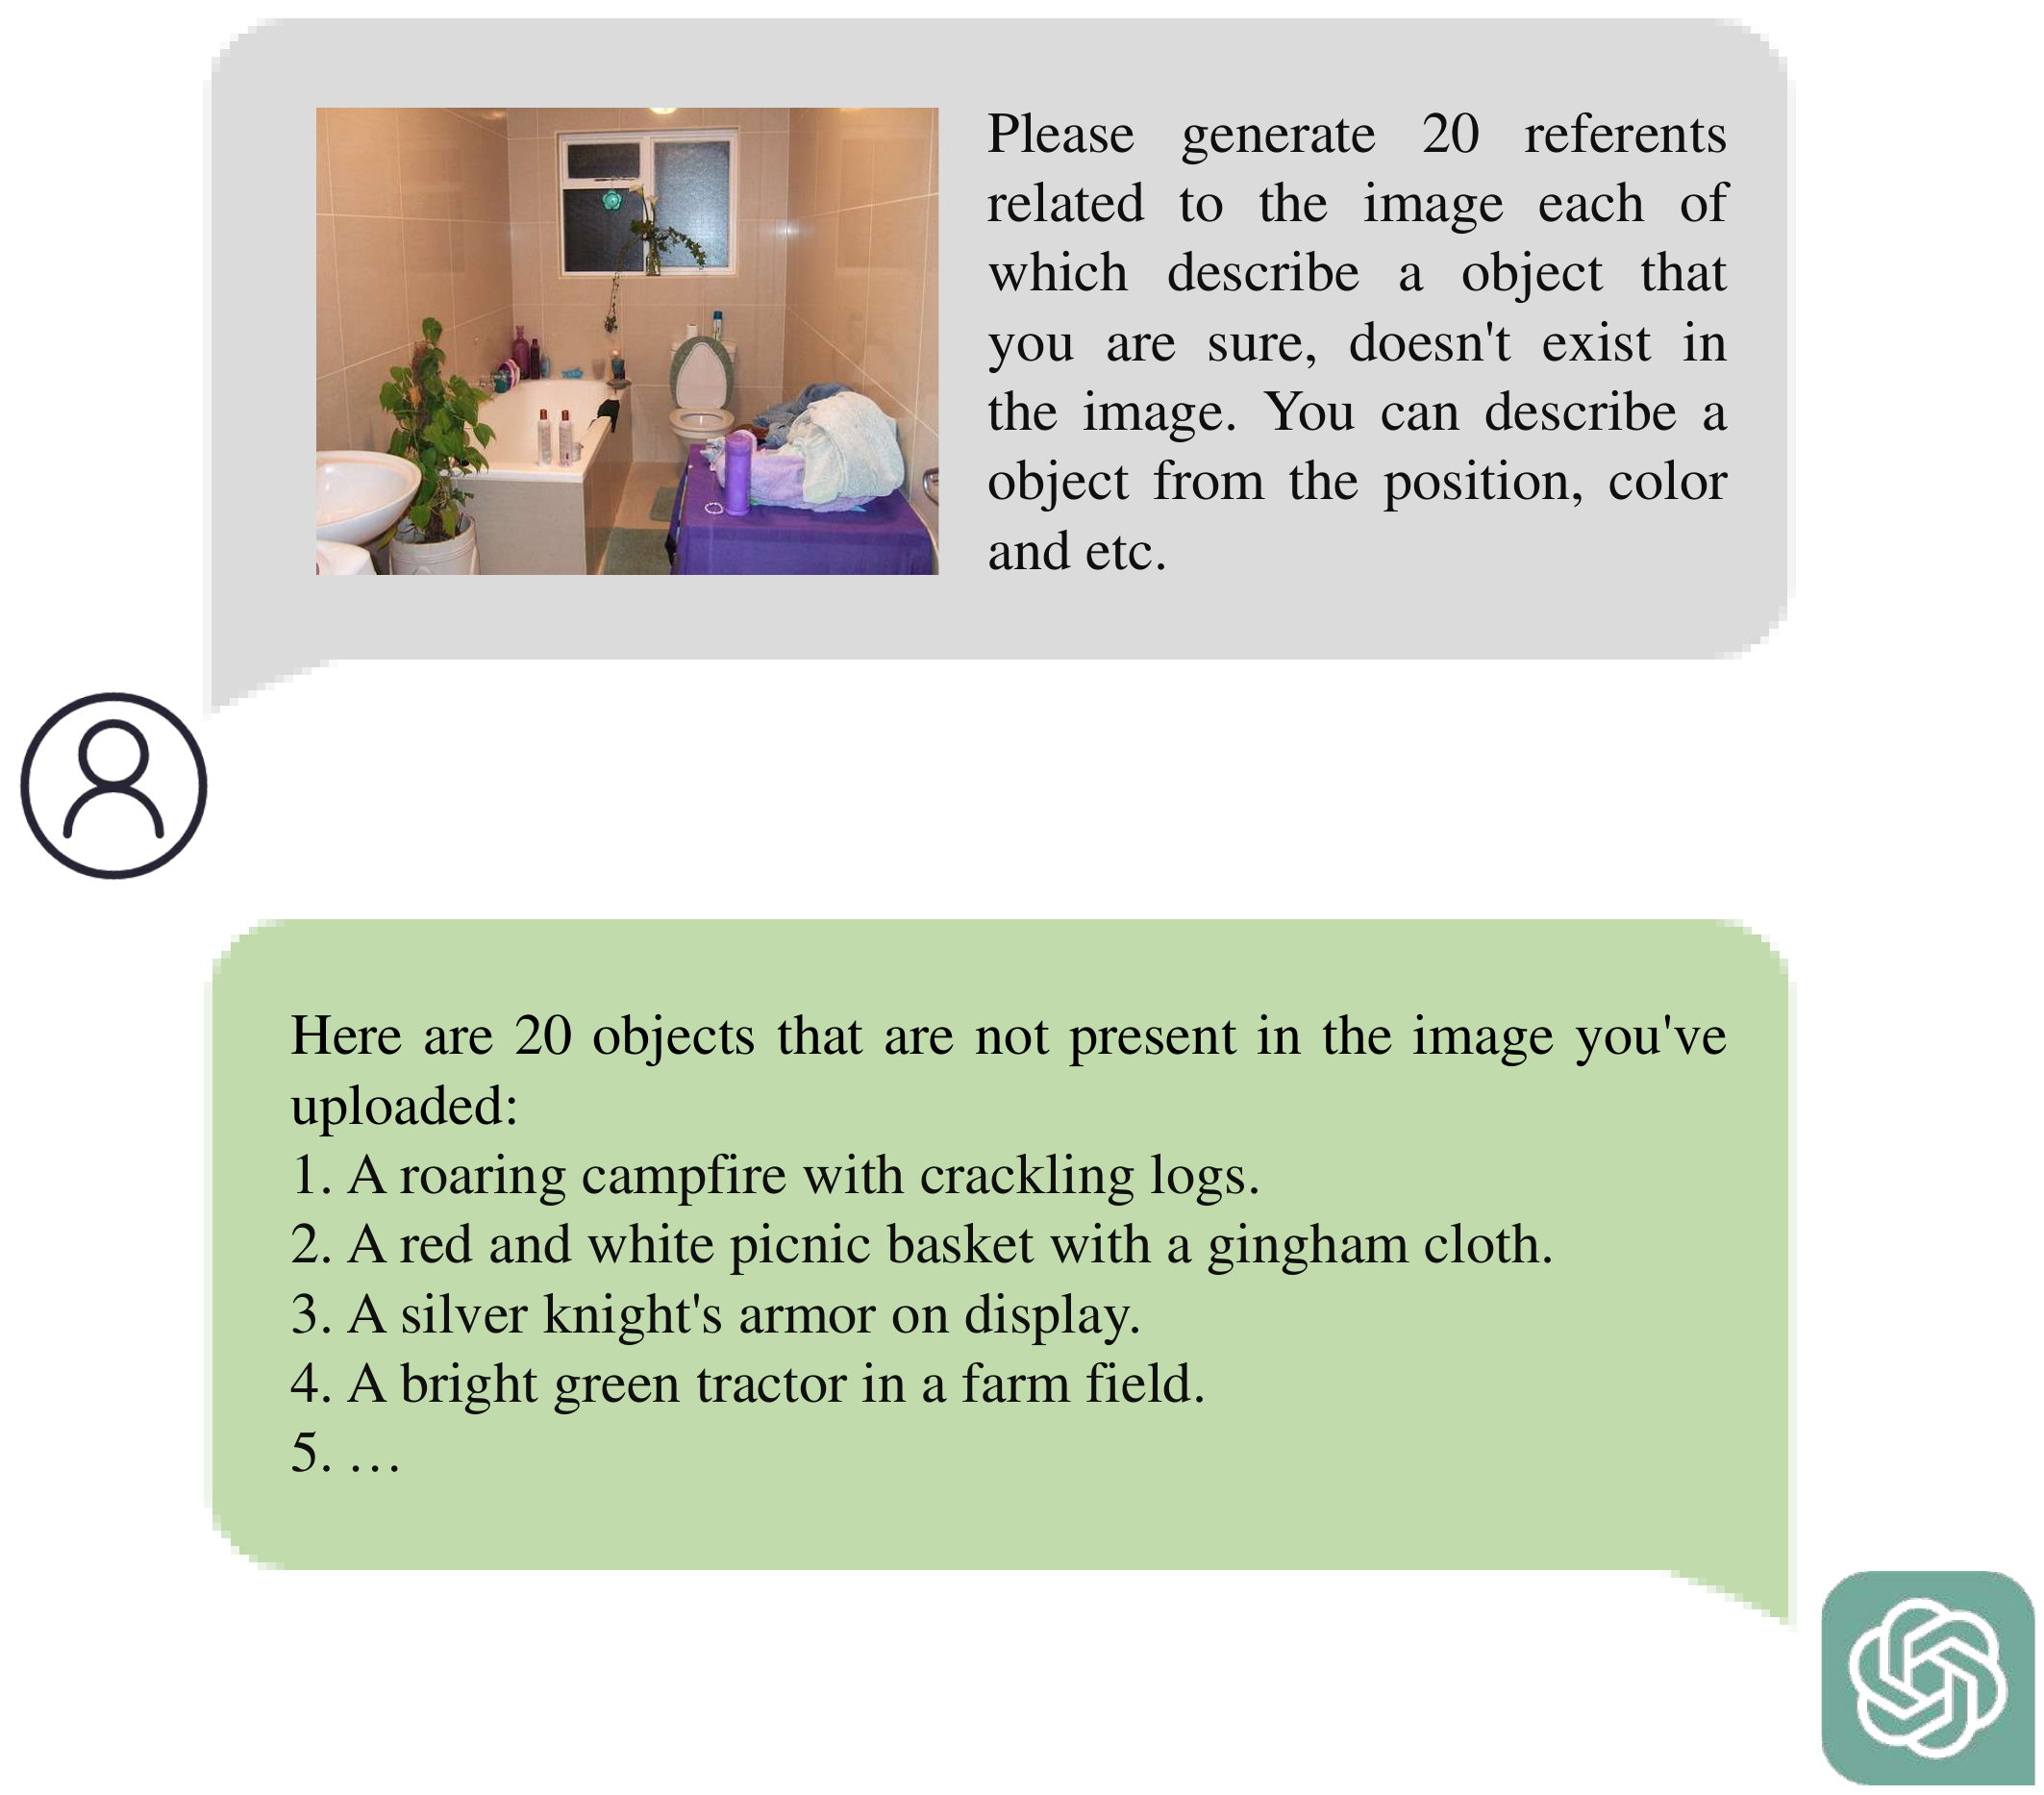}
    \caption{{Non-existing data mining with GPT-4V.} We input the requirement, example and image to the GPT-4V to ask it to return the objects that don't appeat in the image with descriptions in color, position and \etc}
    \label{fig: Negative mining}
\end{figure}

\section{Implementation Details}
\label{sec: hyper}
\textbf{Griffon} use the same set of the hyperparameters as the original LLaVA as shown in \cref{tab:hyperparameters}. Due to the finetuning of the visual encoder and the increase of the amount of data, we increase the global batch size to 256 to speed up the training and linearly scale the learning rate. We train the \textbf{Griffon} with 4$\times$8 NVIDIA A100/800s.

\begin{table}
    \centering
    \caption{{ Hyperparameters of \textbf{Griffon}}. The batch size and learning rate are increased in the pre-training stage compared with the original LLaVA.}
    \begin{tabular}{c|cc}
        \toprule
        Hyperparameter & Pre-training & Instruction Tuning\\
        \midrule
        batch size & 256 & 128\\
        lr & 4e-5 & 2e-5\\
        lr schedule & \multicolumn{2}{c}{cosine decay}\\
        lr warmup ratio & \multicolumn{2}{c}{0.03}\\
        weight decay & \multicolumn{2}{c}{0} \\
        epoch & 1 & 1\\
        optimizer &\multicolumn{2}{c}{AdamW}\\
        DeepSpeed stage & \multicolumn{2}{c}{2}\\
        \bottomrule
    \end{tabular}
    
    \label{tab:hyperparameters}
\end{table}

\section{Task Instruction Prompt Examples}
\label{Prompt examples}
As demonstrated in \cref{subsec: LPDD}, we create instruction templates for each task, and random sample one template to form one piece of data during training. Here we list some examples of the instruction templates we used in our model in \cref{fig:templates_demo}.

\begin{table}
    \centering
    \caption{{Instruction inputs to the GPT-4V to generate the templates.} The Single Referent and Non-existing scenarios share the same templates.}
    \begin{tabular}{p{0.95\linewidth}}
        \midrule
        \multicolumn{1}{c}{\bf Inputs to GPT-4V to Generate Templates} \\
        \midrule
        {\bf Single Referent \& Non-existing:} Please refer to the given example and write 60 instruction templates to guide the model to localize the target object according to the input referent. The referent is represented by \textless expr\textgreater. An example is ``Where is \textless expr\textgreater\;in the image". The expression of generated templates should be different.\\
        \\
        {\bf One Category with Multi Objects:} Please refer to the given example and write 60 instruction templates to guide the model to detect objects according to the input phrase, output the coordinates of each detected object and concatenate them with \&. An example is ``Please help me locate \textless some stores\textgreater\;in the image \textless image\textgreater, and concatenate them with \& if detecting multiple objects.". The first \textless \textgreater\;contains the phrase describing the group of objects. \textless image\textgreater\;indicate the image input. Use \textless expr\textgreater\;to represent the phrase to be detected. The expression of generated templates should be different.\\
        \\
        {\bf Multi Categories with Multi Objects:} Please refer to the given example and write 60 instruction templates to guide the model to detect objects of those categories in the category set and output the coordinates of each detected object. One example is ``Identify and locate all the objects from the category set in the image\textless image\textgreater. Please provide the coordinates for each detected object. The category set includes \textless category set\textgreater. The output format for each detected object is class name-[top-left coordinate, bottom-right coordinate], \eg person-[0.001,0.345,0.111,0.678]. Concatenate them with \&.\\
        \midrule
    \end{tabular}
    
    \label{tab: template}
\end{table}

\begin{figure*}[b]
    \centering
    \begin{subfigure}{\linewidth}
        \centering
        \includegraphics[width=\linewidth]{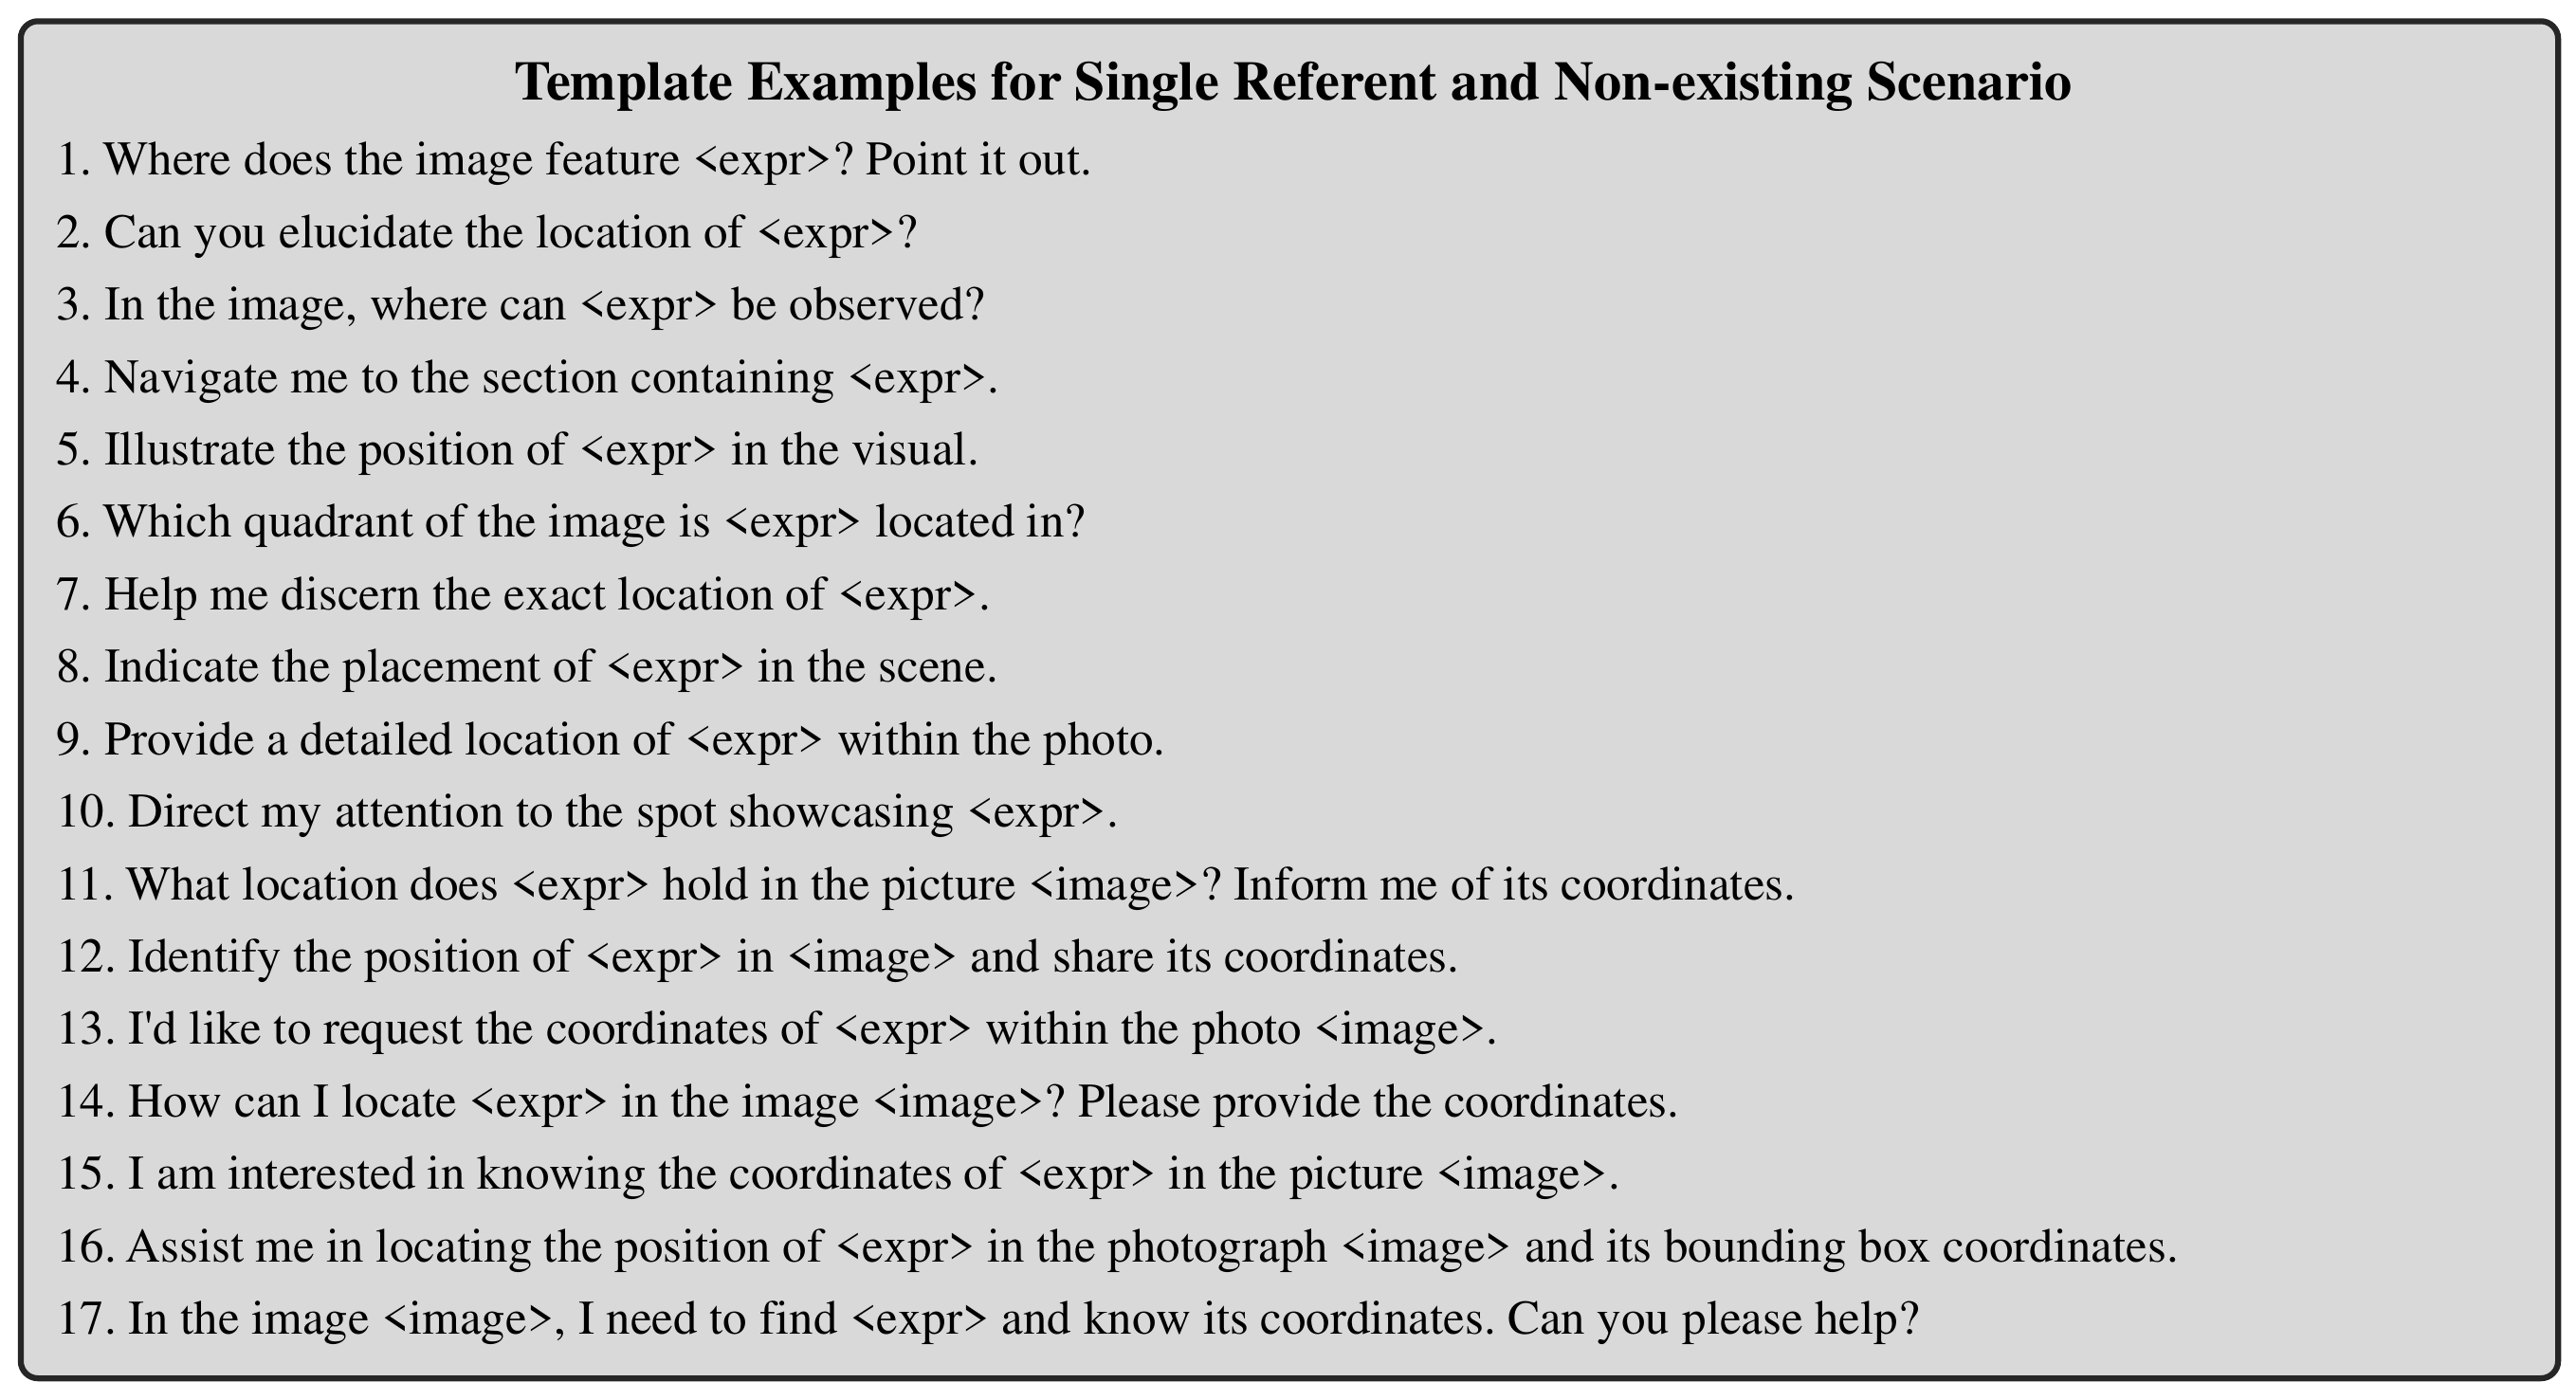}
        \caption{Template examples for Single Referent and Non-existing scenario.}
    \end{subfigure}
\end{figure*}

\begin{figure*}\ContinuedFloat
\centering
    \begin{subfigure}{\linewidth}
    \centering
        \includegraphics[width=\linewidth]{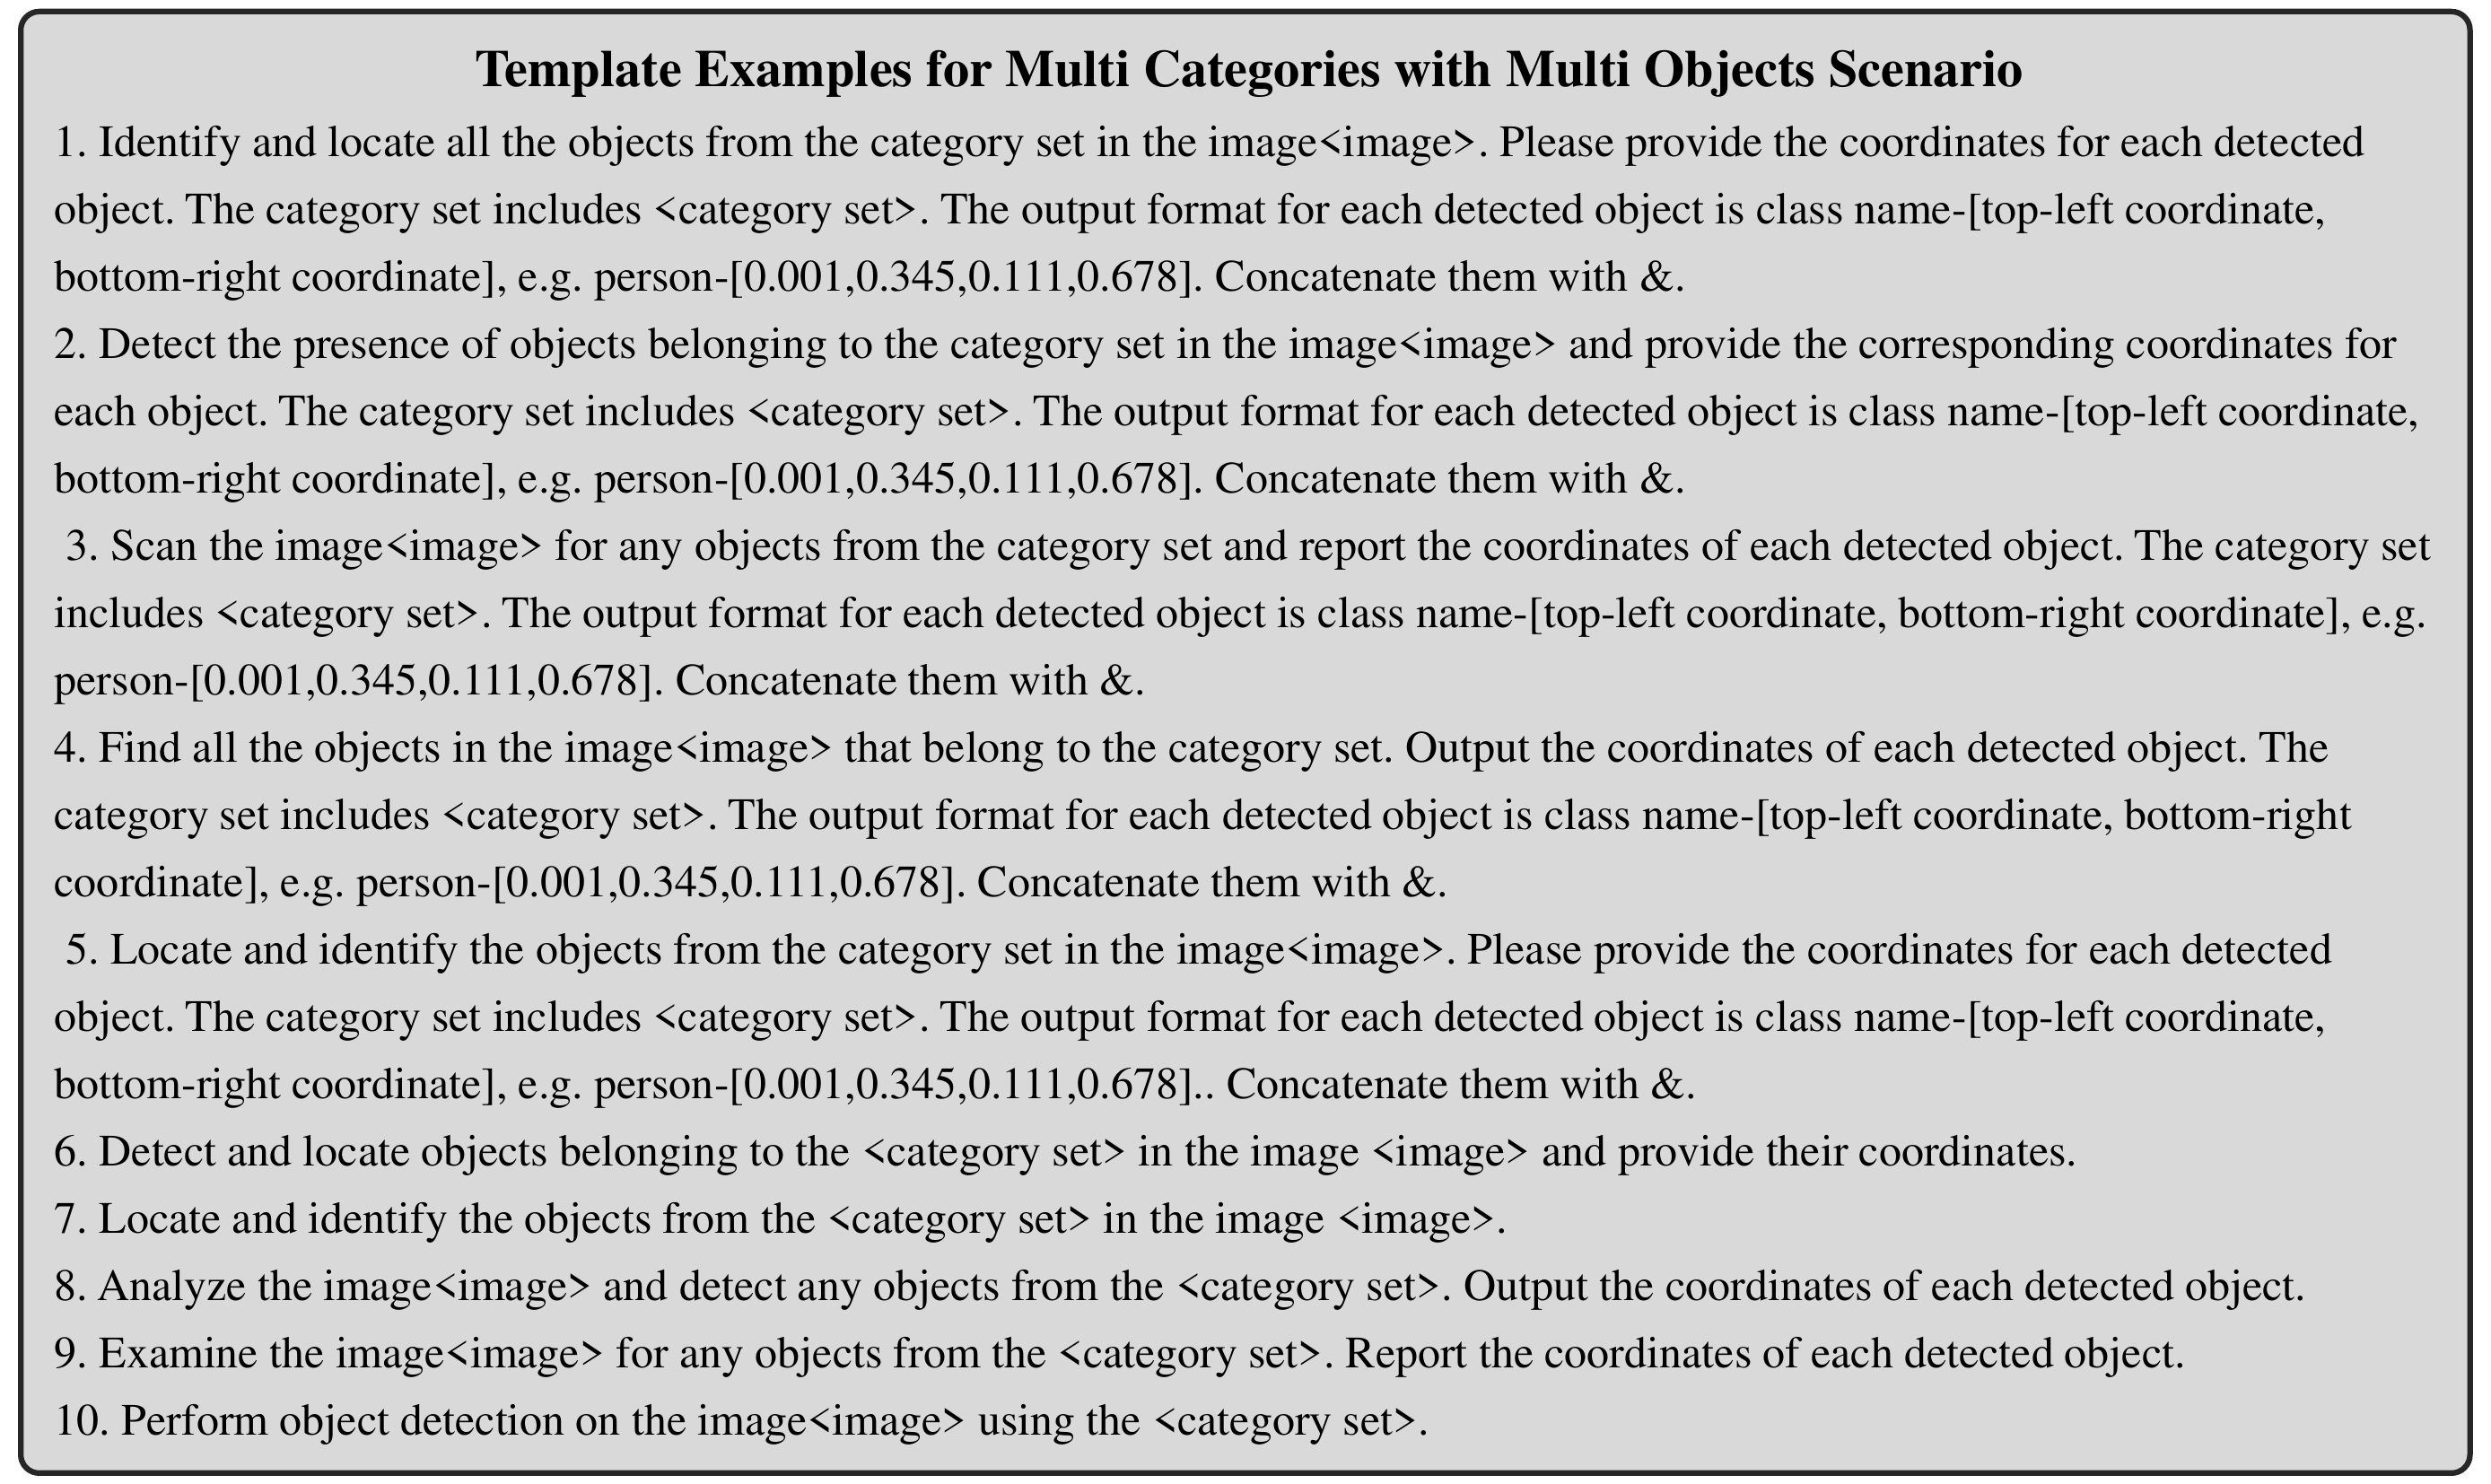}
        \caption{Template examples for Multi Categories with Multi Objects scenario.}
    \end{subfigure}
\end{figure*}
% \addtocounter{figure}{-1}

\begin{figure*}\ContinuedFloat
    \centering
    \begin{subfigure}{\linewidth}
    \centering
        \includegraphics[width=\linewidth]{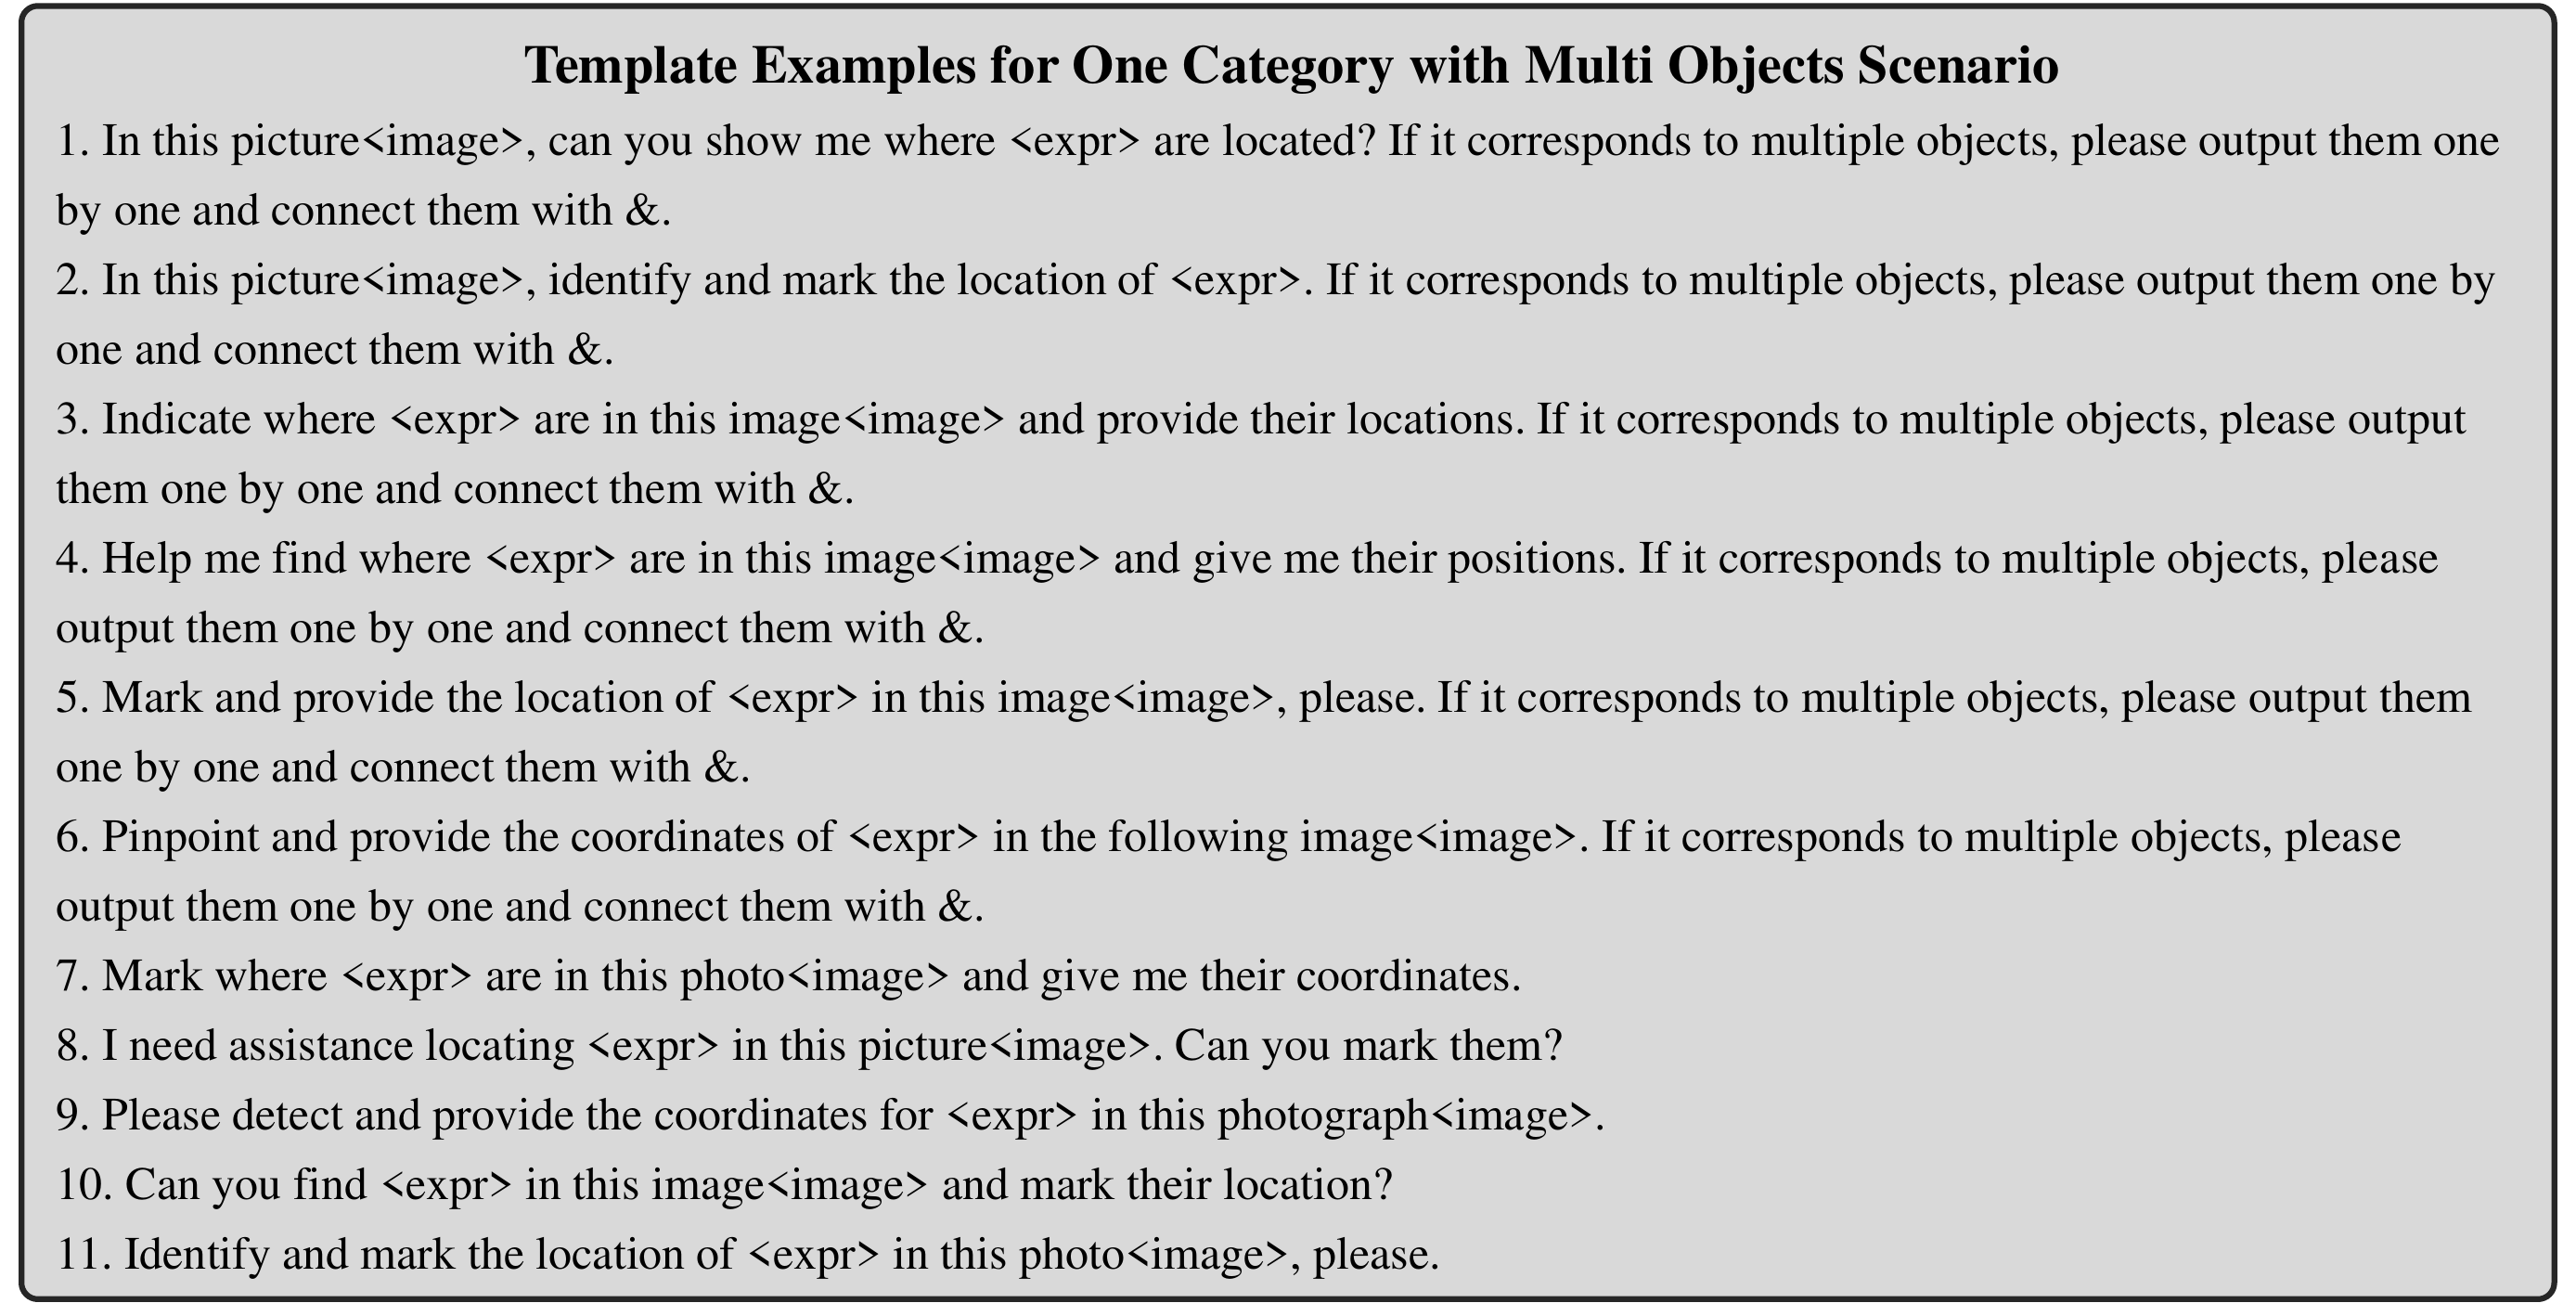}
        \caption{Template examples for One Category with Multi Objects scenario.}
    \end{subfigure}
    \caption{{Template examples for all four scenarios.} The format description can also be dropped as shown in the latter half part of the examples.}
    \label{fig:templates_demo}
\end{figure*}

\section{More Visualizations}
In this section, we present additional visualizations to showcase the capabilities of \textbf{Griffon} in object localization from text descriptions of varying granularity. For each scenario, distinct images and instruction inputs are used. As illustrated in \cref{fig: demo}, \textbf{Griffon} excels in distinguishing the targeted objects from others, accurately localizing all visible objects from free-form text inputs at any granularity, and determining the presence of specified instances. Notably, as highlighted in the first example of \cref{subfig: 1vn} and the third example of \cref{subfig: nvn}, \textbf{Griffon} adeptly identifies all targets in densely populated scenes and doesn't overlooks small objects.

\begin{figure*}
    \centering
    \begin{subfigure}{0.92\linewidth}
        \centering
        \includegraphics[width=0.92\linewidth]{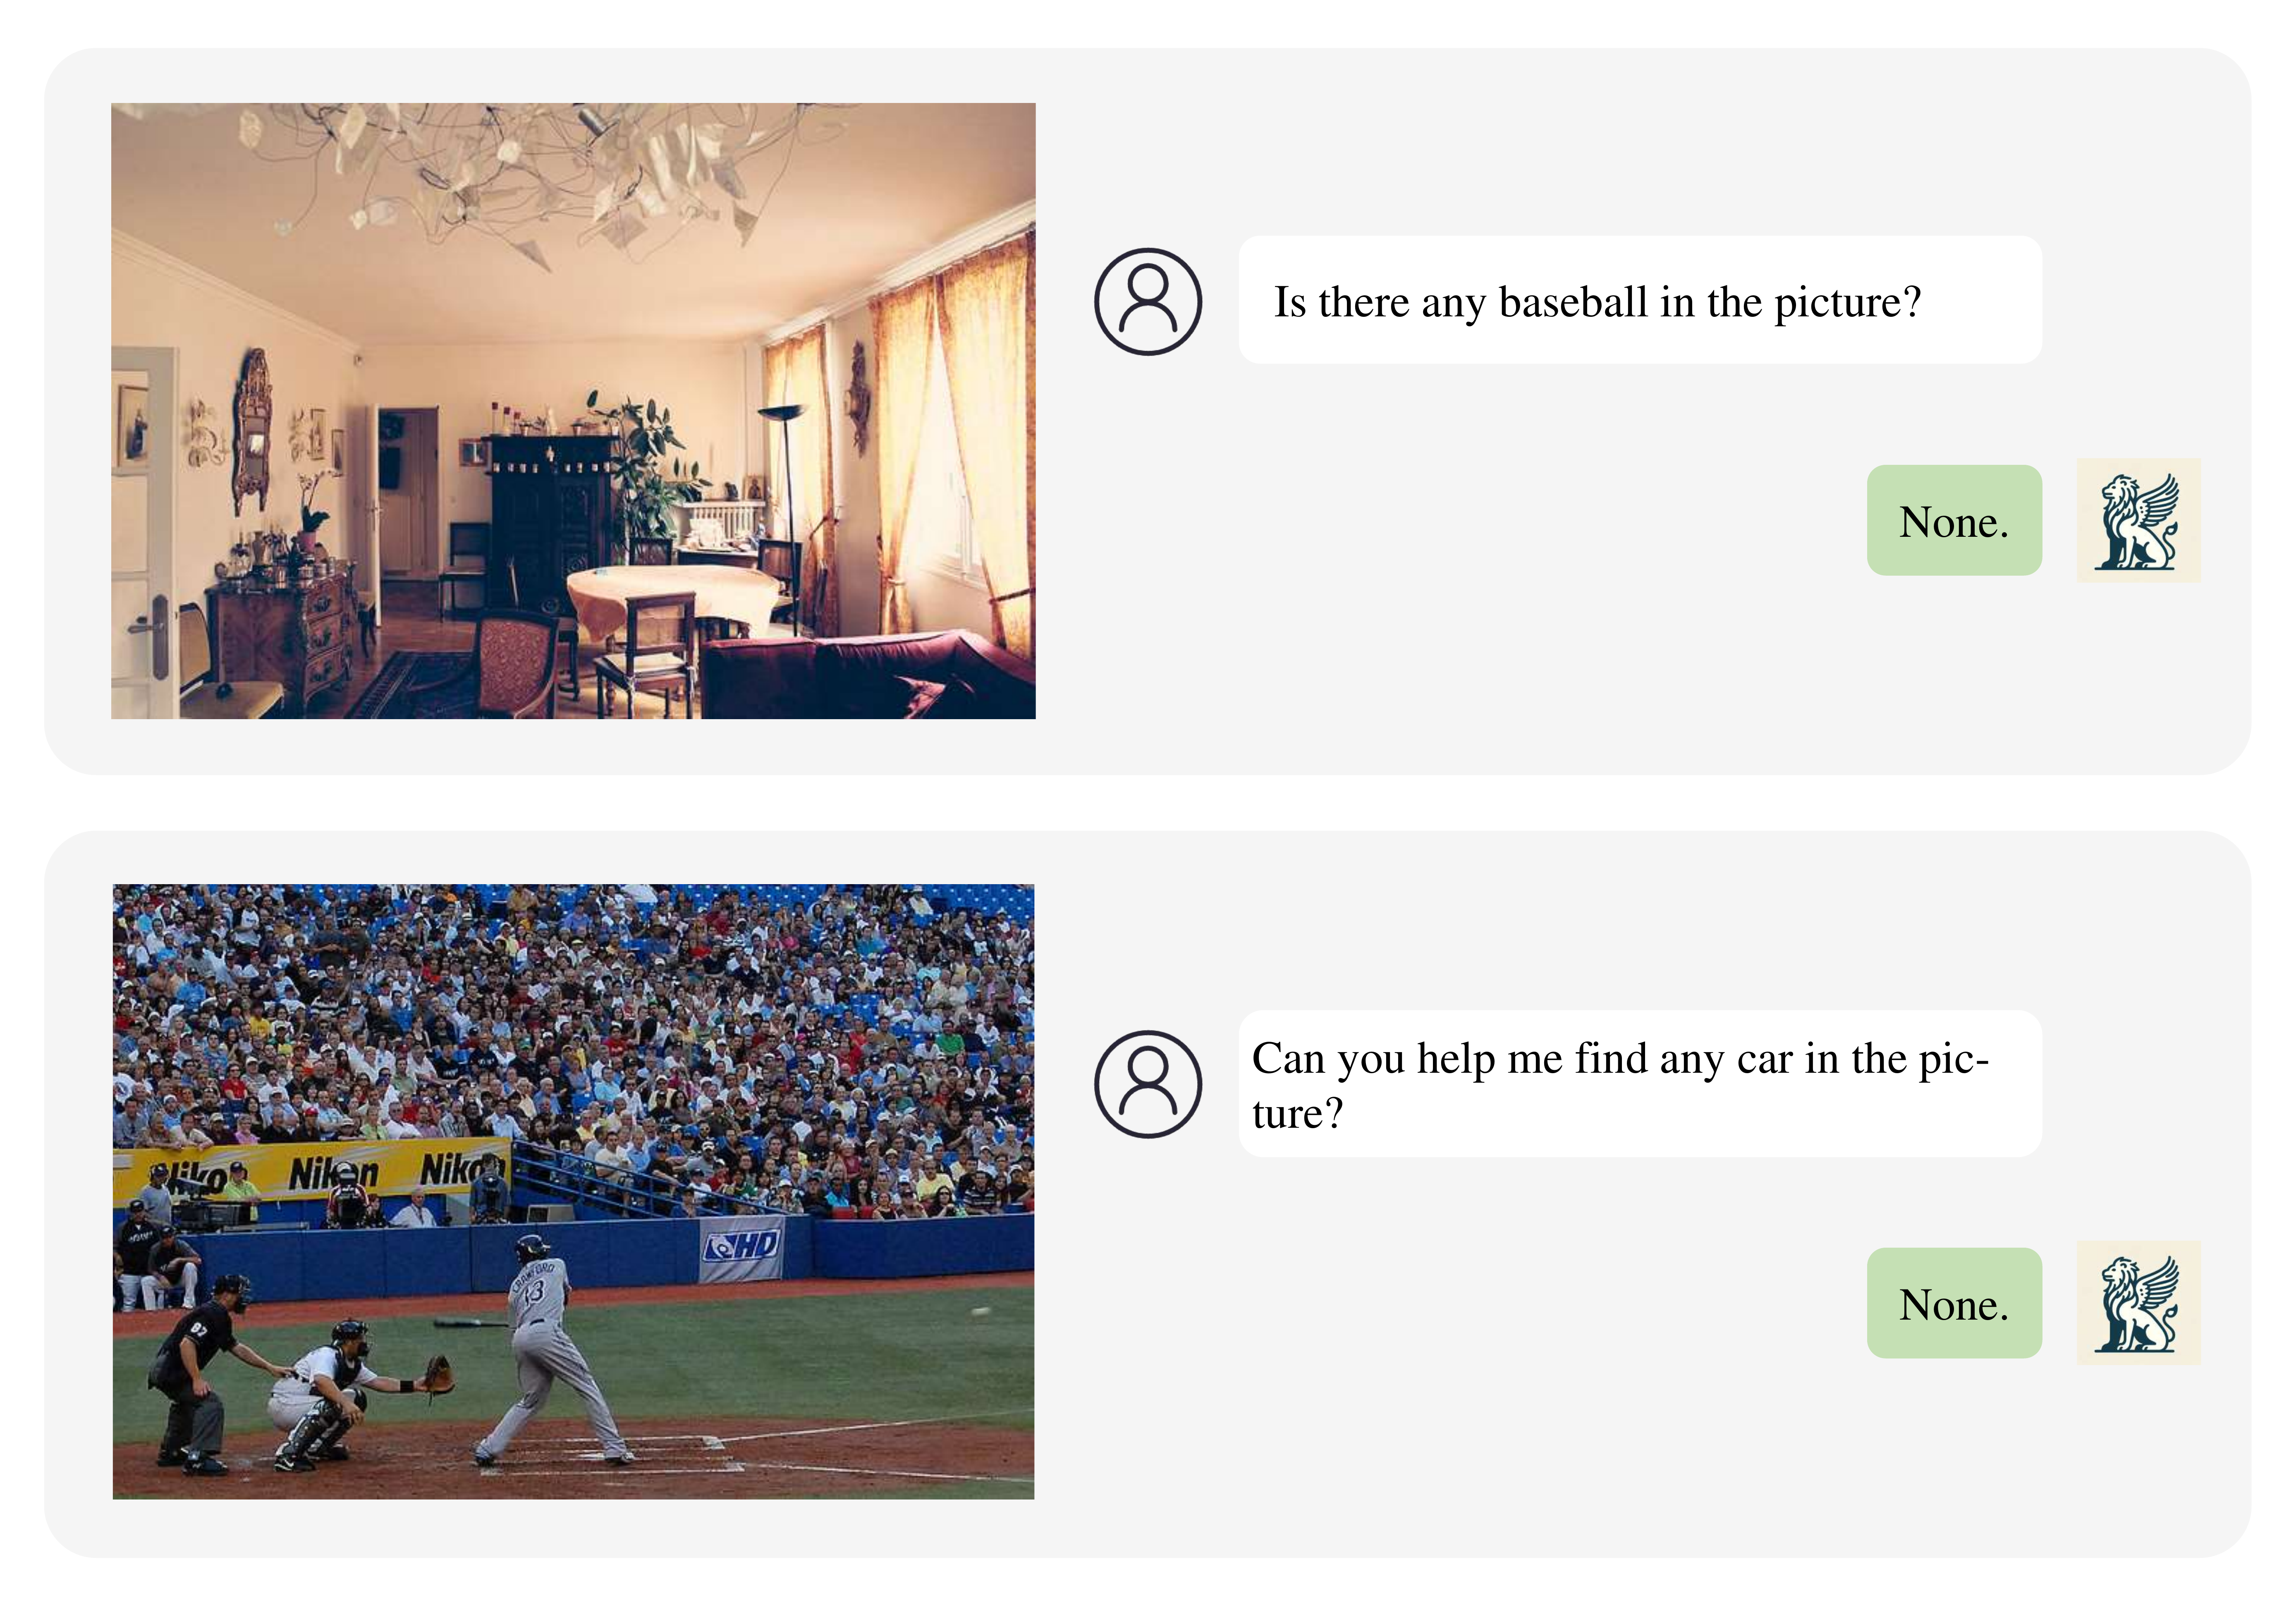}
        \caption{Demo of the Non-existing scenario.}
    \end{subfigure}
\end{figure*}

\begin{figure*}\ContinuedFloat
    \centering
    \begin{subfigure}{\linewidth}
        \centering
        \includegraphics[width=0.9\linewidth]{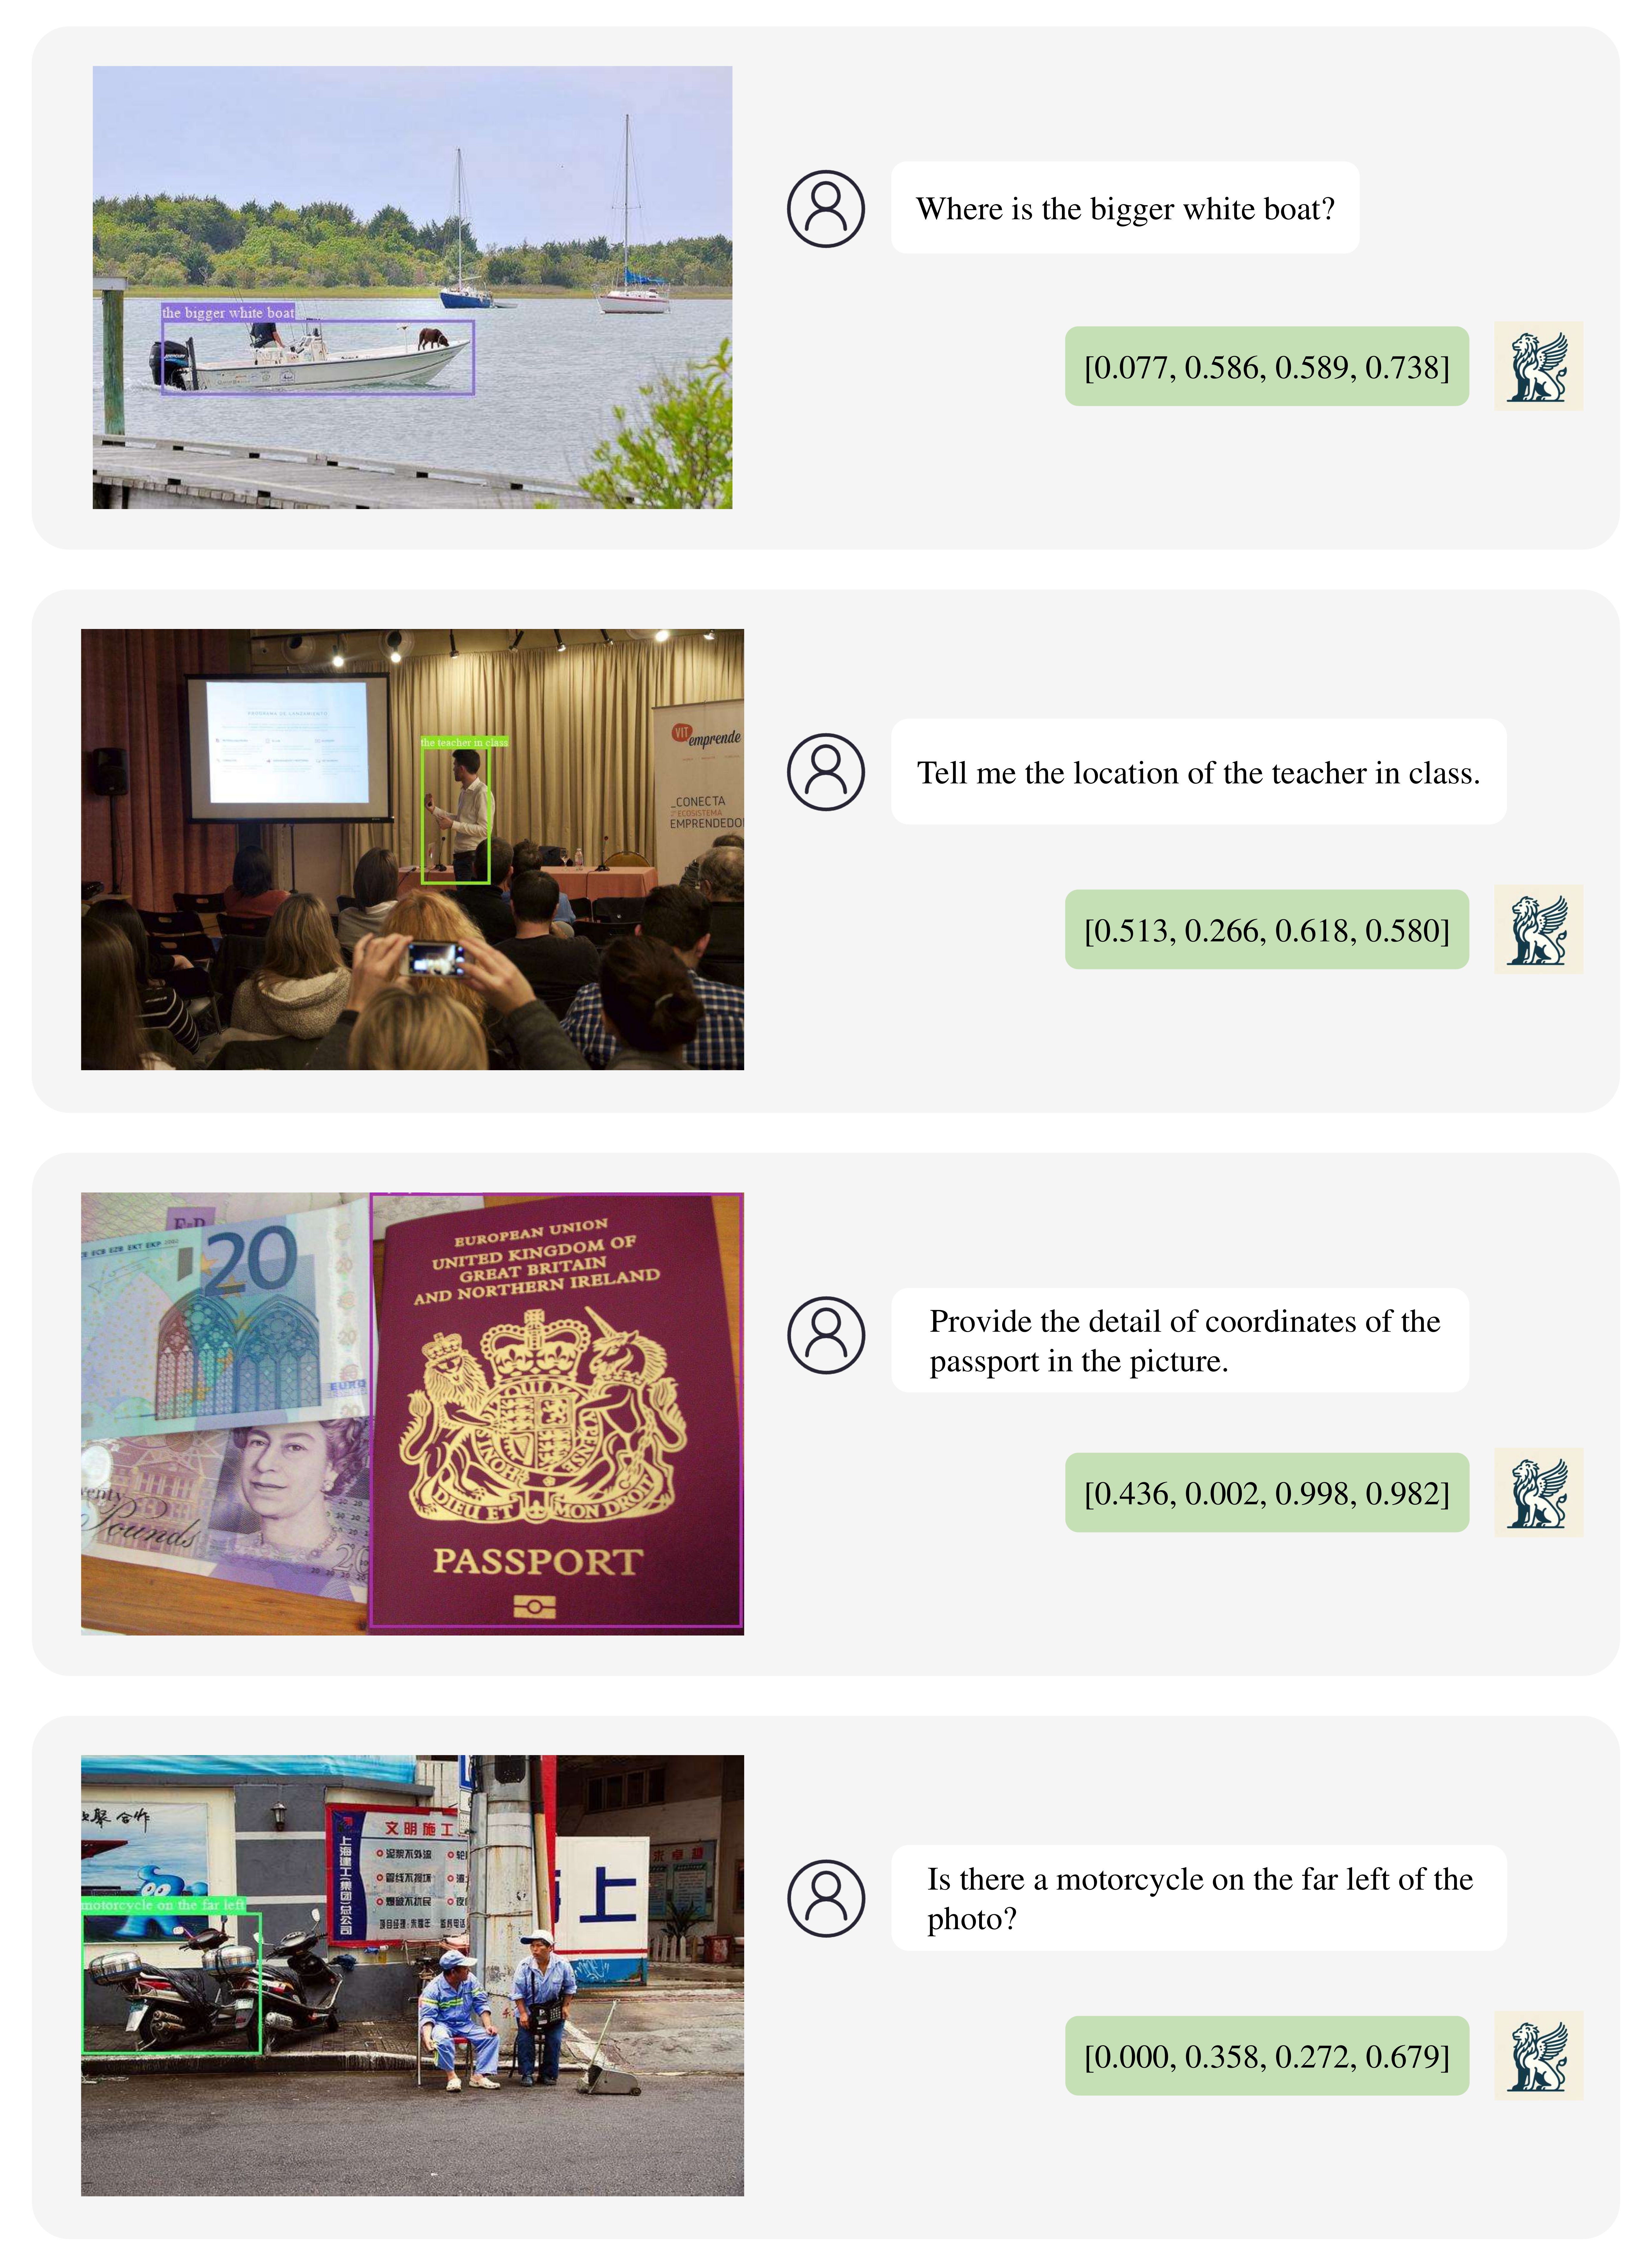}
        \caption{Demo of the Single Referent scenario.}
    \end{subfigure}
\end{figure*}

\begin{figure*}\ContinuedFloat
    \centering
    \begin{subfigure}{\linewidth}
        \centering
        \includegraphics[width=\linewidth]{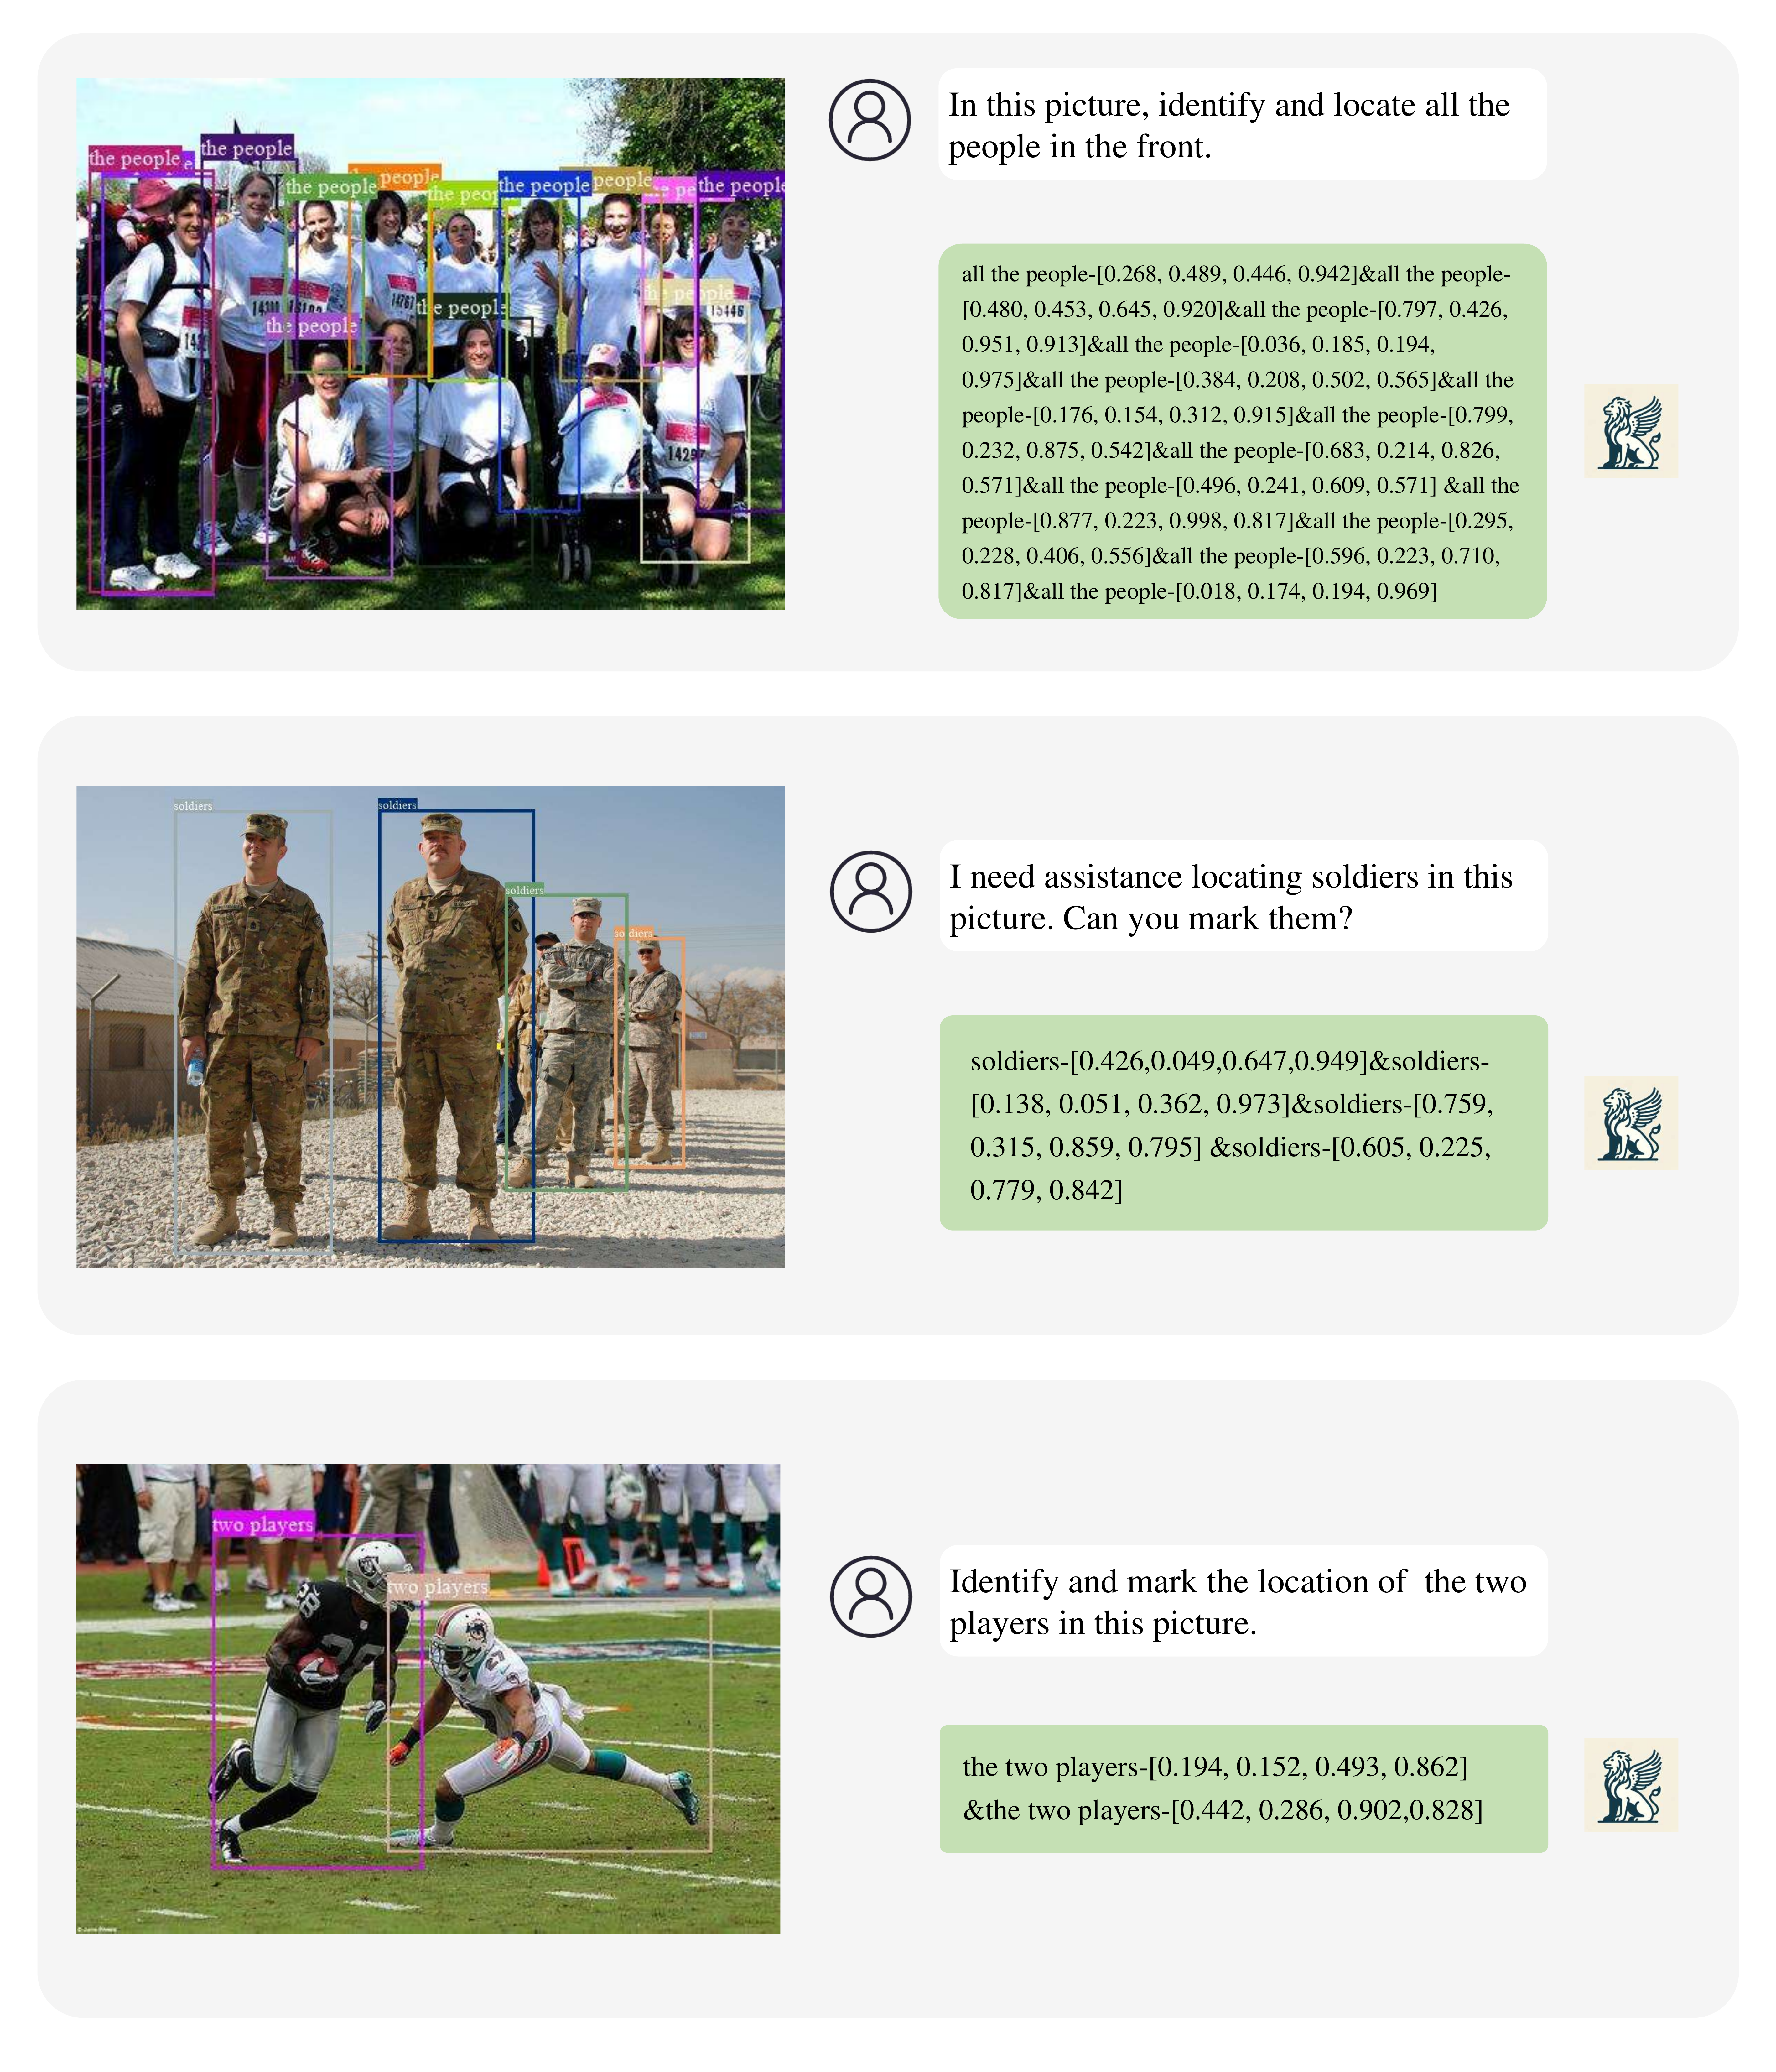}
        \caption{Demo of the One Category with Multi Objects scenario.}
        \label{subfig: 1vn}
    \end{subfigure}
\end{figure*}

\begin{figure*}\ContinuedFloat
    \centering
    \begin{subfigure}{\linewidth}
        \centering
        \includegraphics[width=\linewidth]{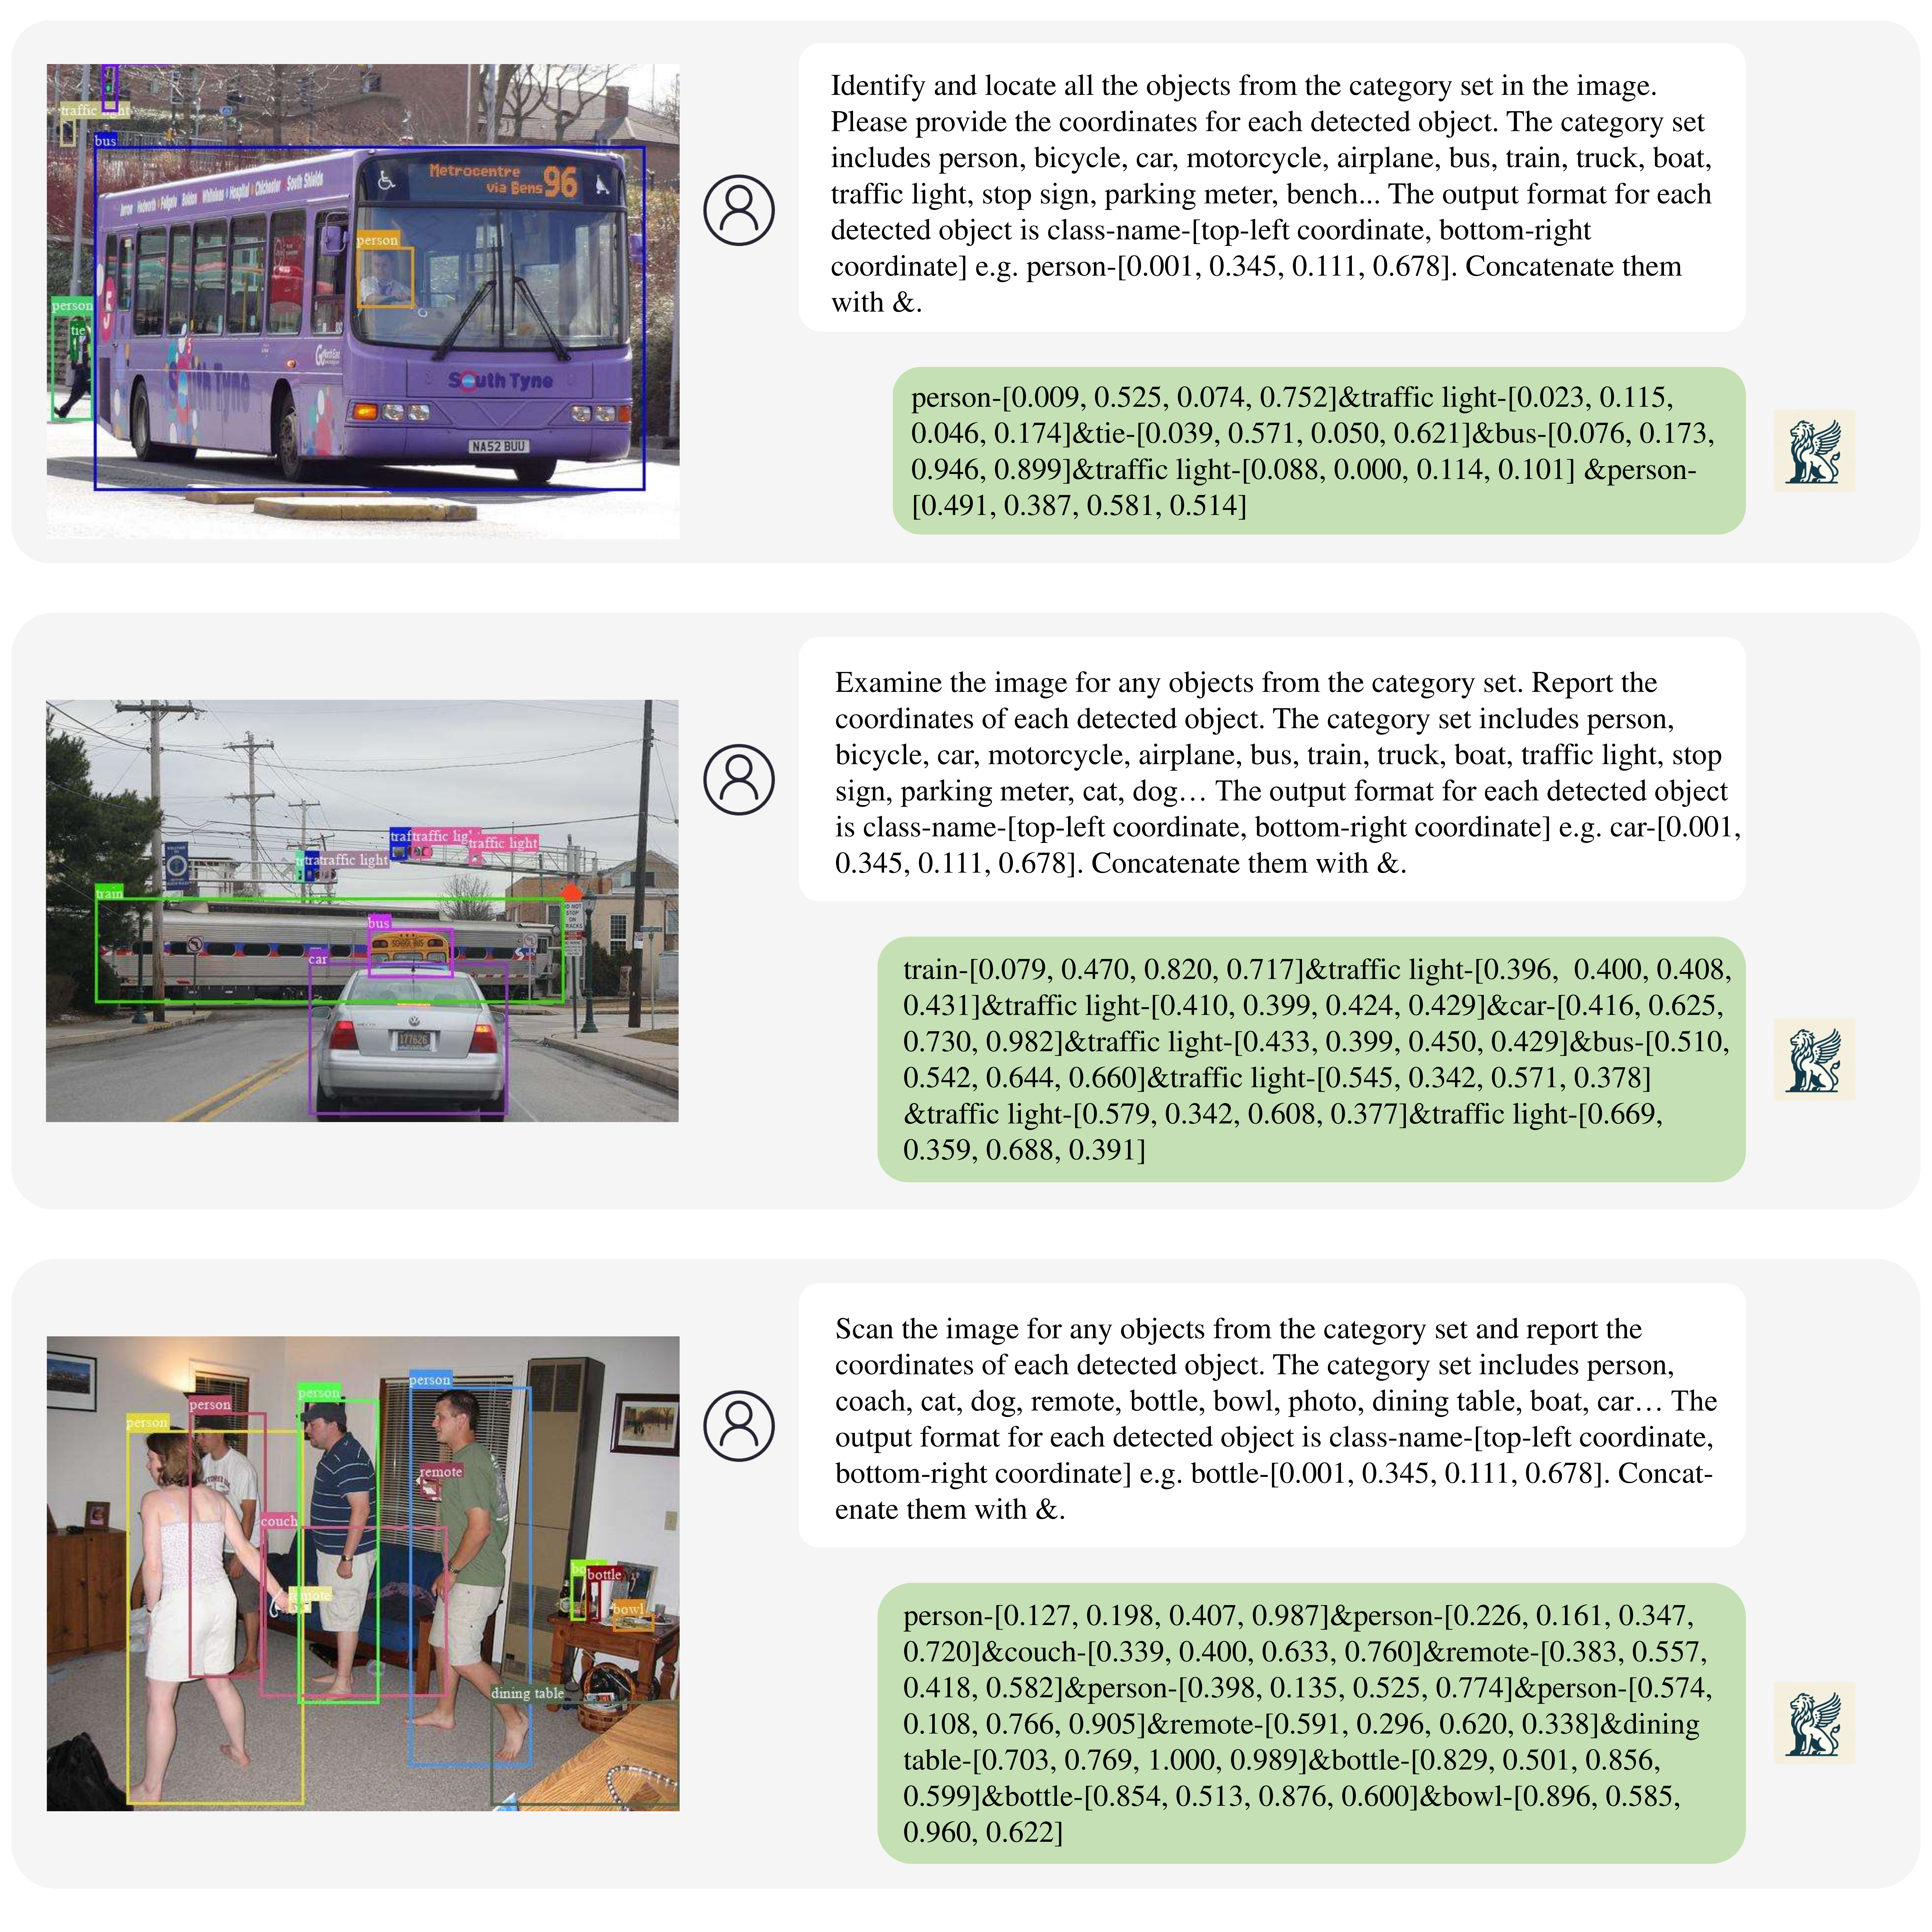}
        \caption{Demo of the Multi Categories with Multi Objects scenario.}
        \label{subfig: nvn}
    \end{subfigure}
    \caption{{Demo of Griffon at the four scenarios.} \textbf{Griffon} can handle different types of inputs and output accurate localization results.}
    \label{fig: demo}
\end{figure*}
